# Supplementary material for: CryoHype: Reconstructing a thousand cryo-EM structures with transformer-based hypernetworks
Source: arXiv:2512.06332 source file (2026-03-19)
Supplement: Supplementary file 2 [file empiar10028.tex]

\begin{table}[!htb]
    \vspace{-8pt}
    \caption{Map-to-model FSC-AUC, \texttt{EMPIAR-10028}}
    \centering
    \label{tab:empiar10028}
    \scalebox{0.85}{
    \begin{tabular}{l|c|c}
        \toprule
        \multirow{2}{*}{\textbf{Method}} & \multicolumn{2}{|c}{\textbf{EMPIAR-10028}} \\
         & Mean $\mathrm{FSC}_{\mathrm{AUC}}$ (std) & Med \\
        \midrule
        CryoDRGN & 0.469 (0.018) & 0.474 \\
        \method/ & 0.479 (0.002) & 0.479 \\
        \bottomrule
    \end{tabular}
    }
\end{table}
\vspace{-10pt}
