# Supplementary material for: CryoHype: Reconstructing a thousand cryo-EM structures with transformer-based hypernetworks
Source: arXiv:2512.06332 source file (2026-03-19)
Supplement: Supplementary file 3 [file iggrl.tex]

\begin{table}[!htb]
    \vspace{-10pt}
    \caption{\textbf{\method/ vs baselines on \texttt{IgG-RL}.}}
    \centering
    \label{tab:iggrl}
    \scalebox{0.85}{
    \begin{tabular}{l|c|c}
        \toprule
        \multirow{2}{*}{\textbf{Method}} & \multicolumn{2}{|c}{\textbf{IgG-RL}} \\
         & Mean $\mathrm{FSC}_{\mathrm{AUC}}$ (std) & Med \\
        \midrule
        CryoDRGN & 0.331 (0.016) & 0.333 \\
        DRGN-AI-fixed & 0.348 (0.012) & 0.350 \\
        Opus-DSD & 0.343 (0.012) & 0.346 \\
        3DFlex & 0.337 (0.007) & 0.337 \\
        3DVA & 0.333 (0.014) & 0.335 \\
        RECOVAR & 0.363 (0.011) & 0.363 \\
        cryoSPARC 3D class & 0.309 (0.006) & 0.307 \\
        \midrule
        \method/ & 0.346 (0.006) & 0.346 \\
        \bottomrule
    \end{tabular}
    }
\end{table}
\vspace{-15pt}
% \begin{table}[htb]
%     \vspace{-10pt}
%     \caption{\method/ vs baselines on IgG-RL}
%     \centering
%     \label{tab:iggrl}
%     \scalebox{0.85}{
%     \begin{tabular}{l|c|c}
%         \toprule
%         \multirow{2}{*}{\textbf{Method}} & \multicolumn{2}{|c}{\textbf{IgG-RL}} \\
%          & Mean $\mathrm{FSC}_{\mathrm{AUC}}$ (std) & Med \\
%         \midrule
%         CryoDRGN~\cite{zhong2021cryodrgn} & 0.331 (0.016) & 0.333 \\
%         DRGN-AI-fixed~\cite{levy2024revealing} & 0.348 (0.012) & 0.350 \\
%         Opus-DSD~\cite{luo2023opus} & 0.343 (0.012) & 0.346 \\
%         3DFlex~\cite{punjani20233dflex} & 0.337 (0.007) & 0.337 \\
%         3DVA~\cite{punjani20213d} & 0.333 (0.014) & 0.335 \\
%         RECOVAR~\cite{gilles2025cryo} & 0.363 (0.011) & 0.363 \\
%         cryoSPARC 3D class~\cite{punjani2017cryosparc} & 0.309 (0.006) & 0.307 \\
%         \midrule
%         \method/ & 0.346 (0.006) & 0.346 \\
%         \bottomrule
%     \end{tabular}
%     \vspace{-10pt}
%     }
% \end{table}
