# Supplementary material for: CryoHype: Reconstructing a thousand cryo-EM structures with transformer-based hypernetworks
Source: arXiv:2512.06332 source file (2026-03-19)
Supplement: Supplementary file 4 [file activations_vis.tex]

\begin{figure}[!h]
  \vspace{-10pt}
  \centering
  \includegraphics[width=0.8\columnwidth]{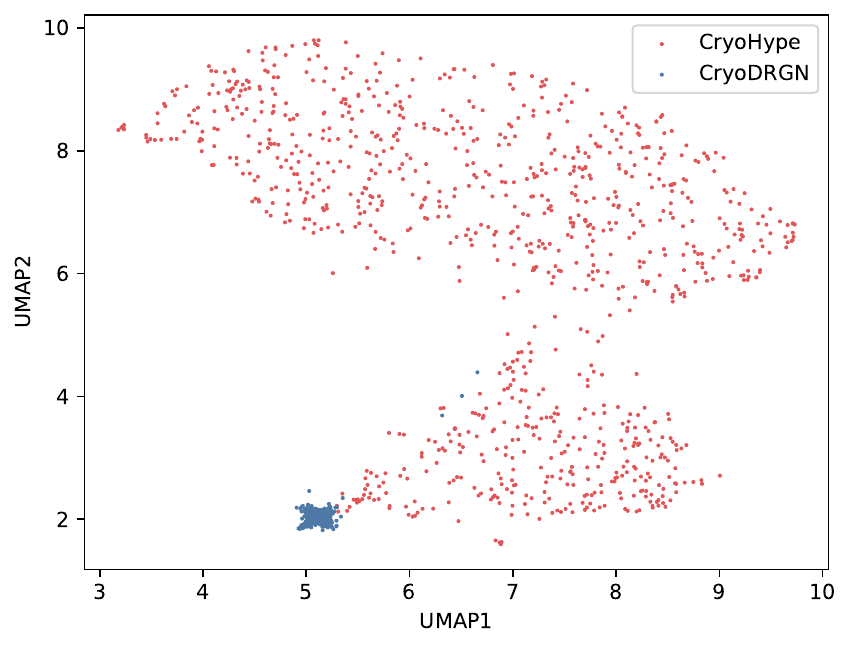}
  \vspace{-10pt}
  \caption{\textbf{Activations of penultimate INR layer, \texttt{Sim2Struct}.} \method/ shows greater diversity in activations. }
  \vspace{-10pt}
  \label{fig:appendix-activations-vis}
\end{figure}

% \begin{figure}[!ht]
%   \vspace{-10pt}
%   \centering
%   \begin{subfigure}{.5\linewidth}
%     \centering
%     \includegraphics[width=.9\linewidth]{Figures/rebuttal/chype_acts3.png}
%     \caption{CryoHype}
%     \label{fig:appendix-acts-vis-cryohype}
%   \end{subfigure}%
%   \begin{subfigure}{.5\linewidth}
%     \centering
%     \includegraphics[width=.9\linewidth]{Figures/rebuttal/cdrgn_acts3.png}
%     \caption{CryoDRGN}
%     \label{fig:appendix-acts-vis-cryodrgn}
%   \end{subfigure}
%   \caption{\textbf{Activations of the fourth INR layer on \texttt{Sim2Struct-1000}.} CryoHype (left) shows much more variation in activations than CryoDRGN (right). Best viewed zoomed in.}
%   \vspace{-10pt}
%   \label{fig:appendix-activations-vis}
% \end{figure}
