# Supplementary material for: CryoHype: Reconstructing a thousand cryo-EM structures with transformer-based hypernetworks
Source: arXiv:2512.06332 source file (2026-03-19)
Supplement: Supplementary file 5 [file empiar10180.tex]

\begin{figure}[!h]
  \vspace{-10pt}
  \centering
  \includegraphics[width=0.8\columnwidth]{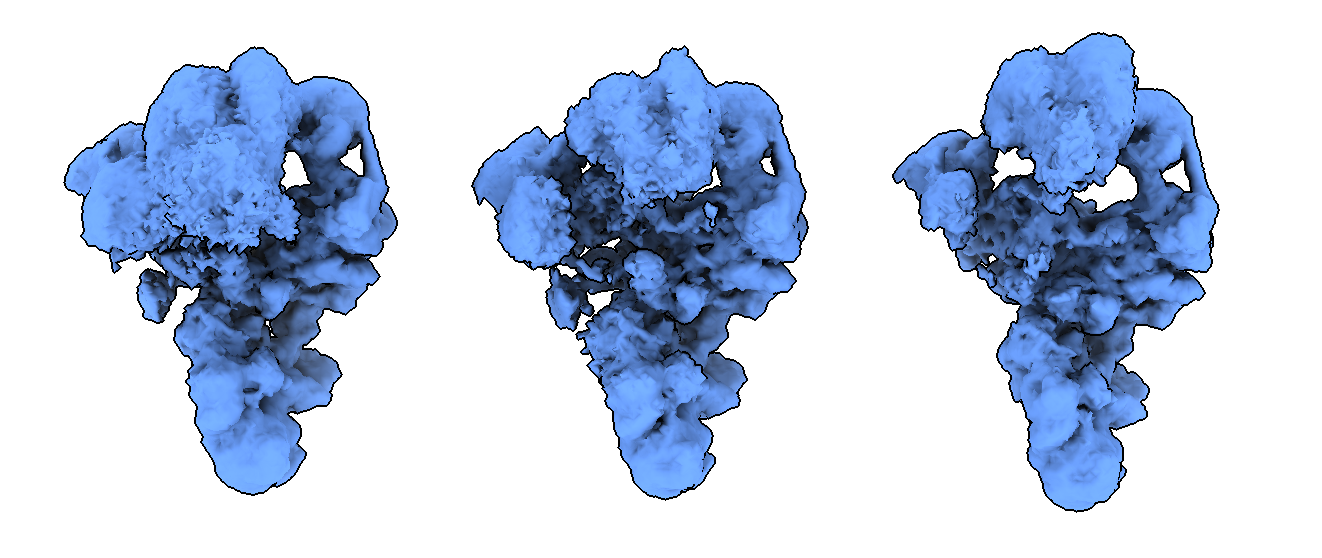}
  \vspace{-10pt}
  \caption{\textbf{\method/ recovers the motion of \texttt{EMPIAR-10180}.}}
  \vspace{-10pt}
  \label{fig:empiar-10180}
\end{figure}
