# Supplementary material for: CryoHype: Reconstructing a thousand cryo-EM structures with transformer-based hypernetworks
Source: arXiv:2512.06332 source file (2026-03-19)
Supplement: Supplementary file 6 [file iggrl_qual_exs.tex]

\begin{figure*}
  \centering
  \includegraphics[width=1.0\linewidth]{Figures/SI/qualitative_IgG-RL.pdf}
  \caption{\textbf{IgG-RL (SNR 0.01) qualitative results} All 100 volumes reconstructed by CryoDRGN (left) and CryoHype (right) for the \texttt{IgG-RL} dataset.}
  \label{fig:si_iggrl}
\end{figure*}
