# Supplementary material for: CryoHype: Reconstructing a thousand cryo-EM structures with transformer-based hypernetworks
Source: arXiv:2512.06332 source file (2026-03-19)
Supplement: Supplementary file 7 [file iggrl_qualitative_metric_comparison.tex]

\begin{figure}
  \centering
  \includegraphics[width=0.9\linewidth]{Figures/SI/metric_figures_iggrl.pdf}
  \caption{\textbf{Qualitative Metric Comparison for IgG-RL (SNR 0.01).} For this structure, all metrics indicate that CryoHype outperforms CryoDRGN. Per-image FSC performance improves by 14$\%$ (from 0.313 to 0.358), while vIoU improves by 57$\%$, and CD improves by 90$\%$. This suggests that the structural differences, particularly CryoDRGN's inability to reconstruct the randomly oriented Fab region, are better captured by the CD and vIoU metrics than in per-image FSC.}
  \label{fig:si_metric_comp_iggrl}
\end{figure}
