# Supplementary material for: CryoHype: Reconstructing a thousand cryo-EM structures with transformer-based hypernetworks
Source: arXiv:2512.06332 source file (2026-03-19)
Supplement: Supplementary file 9 [file s2s_fsc_curves.tex]

\begin{figure*}
  \centering
  \includegraphics[width=1.0\linewidth]{Figures/SI/cryohype_all_fsc_curves_s2s.pdf}
  \caption{\textbf{Per-Image FSC curves for the 10, 100, 200, and 500 structure subsets of \dataset/}}
  \label{fig:si_per-img_fsc_s2s}
\end{figure*}
