# Supplementary material for: CryoHype: Reconstructing a thousand cryo-EM structures with transformer-based hypernetworks
Source: arXiv:2512.06332 source file (2026-03-19)
Supplement: Supplementary file 10 [file shapenet_em_examples.tex]

\begin{figure*}
  \centering
  \includegraphics[width=0.8\linewidth]{author-kit-CVPR2025-v3.1-latex-/images/all_shapenet_em.png}
  \caption{\textbf{ShapeNet-EM.} In this figure, we show all 100 shapes in our \texttt{ShapeNet-EM} dataset. Note that imperfect voxelization results in imperfect shapes.}
  \label{fig:appendix-all-shapenet}
\end{figure*}
