# Supplementary material for: CryoHype: Reconstructing a thousand cryo-EM structures with transformer-based hypernetworks
Source: arXiv:2512.06332 source file (2026-03-19)
Supplement: Supplementary file 11 [file shapenet_em_fsc_curves.tex]

\begin{figure}
  \centering
  \includegraphics[width=1.0\linewidth]{Figures/SI/per-image_FSC_ShapeNet.pdf}
  \caption{\textbf{Per-Image FSC curves for ShapeNet-EM.}}
  \label{fig:si_per-img_fsc_shape}
\end{figure}
