# Supplementary material for: CryoHype: Reconstructing a thousand cryo-EM structures with transformer-based hypernetworks
Source: arXiv:2512.06332 source file (2026-03-19)
Supplement: Supplementary file 12 [file tomo_fsc_cuves.tex]

\begin{figure*}
  \centering
  \includegraphics[width=0.8\linewidth]{Figures/SI/cryohype_all_fsc_curves_tt100.pdf}
  \caption{\textbf{Per-Image FSC curves for Tomotwin-100.}}
  \label{fig:si_per-img_fsc_tomo}
\end{figure*}
