# Supplementary material for: CryoHype: Reconstructing a thousand cryo-EM structures with transformer-based hypernetworks
Source: arXiv:2512.06332 source file (2026-03-19)
Supplement: Supplementary file 13 [file tomo_qualitative_metric_comparison.tex]

\begin{figure*}
  \centering
  \includegraphics[width=0.9\linewidth]{Figures/SI/metric_figures_tomo.pdf}
  \caption{\textbf{Qualitative Metric Comparison for Tomotwin-100 (SNR 0.01).} (a) Both CryoDRGN and CryoHype are capable of reconstructing the overall shape of the protein; however, CryoHype captures high-resolution details better than CryoDRGN. The per-image FSC improves by 13$\%$ (from 0.357 to 0.405), whereas vIoU and CD improve by less than 2$\%$. This indicates that per-image FSC is more sensitive to high-resolution details than vIoU and CD. (b) CryoDRGN fails to capture the shape of the protein, while CryoHype does a much better job of capturing the shape. For CryoHype, the per-image FSC improves over that of CryoDRGN by 11$\%$ (from 0.356 to 0.402), while vIoU and CD exhibit much larger improvements of 140$\%$ and 86$\%$, respectively. This indicates that vIoU and CD are significantly more sensitive to structural differences than per-image FSC.}
  \label{fig:si_metric_comp_tomo}
\end{figure*}
