# Supplementary material for: CryoHype: Reconstructing a thousand cryo-EM structures with transformer-based hypernetworks
Source: arXiv:2512.06332 source file (2026-03-19)
Supplement: Supplementary file 14 [file weights_vis.tex]

\begin{figure}[!ht]
  \vspace{-10pt}
  \centering
  \includegraphics[width=0.9\linewidth]{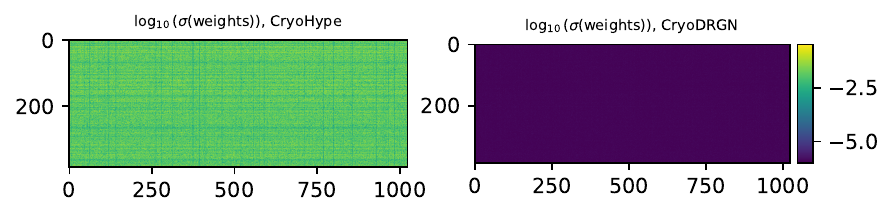}
  \vspace{-10pt}
  \caption{\textbf{Standard deviations of weights and biases of the first INR layer, \texttt{Sim2Struct-1000}.} CryoHype shows much more variation in INR weights than CryoDRGN, which only varies in the biases (last row). Best viewed zoomed in. }
  \label{fig:appendix-weight-vis}
  \vspace{-10pt}
\end{figure}
